# Supplementary material for: eT 1.0: an open source electronic structure program with emphasis on coupled cluster and multilevel methods
Source: arXiv:2002.05631 source file (2020-02-13)
Supplement: Supplementary file 1 [file eT_paper_AIP_SI.pdf]

# Supporting information for "e$^T$ 1.0: an open source electronic structure program with emphasis on coupled cluster and multilevel methods"

## QM/FQ computational details

QM/MM calculations are performed on 64 uncorrelated snapshots extracted from a classical molecular dynamics (MD) simulation in Ref. 1. For each snapshot, a sphere centered on the solute with a radius of 15 Å containing approximately 400 water molecules was extracted from the MD calculation. The UV/Vis spectrum was then calculated, treating PNA at the CC2/aug-cc-pVDZ level and modelling the water molecules with an FQ force field. Two different FQ parametrizations were used: QM/FQ$^a$ from Ref. 2 and QM/FQ$^b$ from Ref. 3.

## TD-CC computational details

The interaction of the water molecule with a $B_1$-polarized UV pulse was calculated for $t \in [0, 320]$ a.u., starting from the time independent coupled cluster ground state at $t = 0$ a.u. The pulse was given a central frequency equal to the first CCSD excitation energy, a peak field strength of 0.01 a.u., and a Gaussian envelope centered at $t = 160$ a.u. with a root mean square width of 10 a.u. After the interaction, we compute Fourier transforms of the time-dependent dipole moments in the $x$-, $y$- and $z$-directions in the interval $t \in [320, 5320]$ a.u. The total absorption spectrum is then obtained by taking the square root of the sum of squared $x$-, $y$- and $z$-direction intensities for each frequency in the Fourier series. For the X-ray spectrum, the central frequency was instead set to the first CCSD/CVS excitation energy, and the pulse given an $A_1$-polarization.

## REFERENCES

[1]T. Giovannini, R. R. Riso, M. Ambrosetti, A. Puglisi, and C. Cappelli, "Electronic transitions for a fully QM/MM approach based on fluctuating charges and fluctuating dipoles: Linear and corrected linear response regimes," J. Chem. Phys. **151**, 174104 (2019).

[2]S. W. Rick, S. J. Stuart, and B. J. Berne, "Dynamical fluctuating charge force fields: Application to liquid water," J. Chem. Phys. **101**, 6141–6156 (1994).

[3]T. Giovannini, P. Lafiosca, B. Chandramouli, V. Barone, and C. Cappelli, "Effective yet reliable computation of hyperfine coupling constants in solution by a QM/MM approach: Interplay between electrostatics and non-electrostatic effects," J. Chem. Phys. **150**, 124102 (2019).
